# Supplementary material for: Experimental and ab initio ultrafast carrier dynamics in plasmonic nanoparticles
Source: arXiv:1608.03309 source file (2016-12-24)
Supplement: Supplementary file 1 [file SI.pdf]

# Supplemental Information for:
# Ultrafast carrier experimental and *ab initio* dynamics in plasmonic nanoparticles

Ana M. Brown,[1] Ravishankar Sundararaman,[2] Prineha Narang,[1,2,3] Adam Schwartzberg,[4] William A. Goddard III,[2,5] and Harry A. Atwater[1,2]

[1]*Thomas J. Watson Laboratories of Applied Physics, California Institute of Technology*
[2]*Joint Center for Artificial Photosynthesis, California Institute of Technology*
[3]*NG NEXT, 1 Space Park Drive, Redondo Beach CA*
[4]*The Molecular Foundry, Lawrence Berkeley National Laboratory, 1 Cyclotron Road, Berkeley CA*
[5]*Materials and Process Simulation Center, California Institute of Technology, 1200 East California Blvd, Pasadena CA 91125 USA*

(Dated: December 12, 2016)

## SPATIAL DYNAMICS OF ELECTRONS

As experimental systems for ultrafast spectroscopy of metals, both thin films and nanoparticles have distinct advantages and disadvantages. Thin films are in general a cleaner system, offering potentially much better control over geometry, surface quality and grain-size / crystallinity. However, modelling and interpreting ultrafast spectroscopy of these systems involves one additional complication: the electron distributions vary in space as well as in time. Within the two temperature model, the spatial variation is usually handled via an electron thermal conductivity term, but this description is only valid over length scales much larger than the characteristic mean free path on the order of tens of nanometers. At intermediate dimensions, super-diffusive and ballistic electron transport effects become important.

On the other extreme, in plasmonic nanoparticles with dimensions on the order of these mean free paths and smaller, the carrier distributions remain spatially homogeneous to an excellent approximation. We therefore pick such plasmonic particles for a first joint experimental and *ab initio* study. Neglecting the spatial dependence allows us to treat the time dynamics and spectral response in much greater detail with electronic structure methods, than previously possible with empirical free-electron models.

Extending such an analysis to the case with spatial transport is the subject of future work. This requires adding spatial degrees of freedom to the Boltzmann equation, and computing the *ab initio* collision integrals as we do here, separately for different points in space. This level of theory will naturally capture super-diffusive / ballistic transport as well as energy-dependence of the carrier mean free paths. Although the theoretical formulation to include spatial dependence is straightforward, the computational expense increases substantially, requiring development of appropriate algorithms to make such calculations practical.

## ELECTRON-PHONON COLLISION INTEGRAL

We need to calculate the electron-phonon collision integral for the interaction of an arbitrary hot electron distribution, $f(\varepsilon)$, with a thermal phonon distribution $n(\omega, T_l)$, given by the Bose distribution at lattice temperature $T_l$. We start with the rate of energy transfer between the electrons and lattice per unit volume, which is exactly (6) and (7) from Ref. 1, except that we allow $f(\varepsilon)$ to be an arbitrary distribution (instead of restricting it to a Fermi distribution at some temperature $T_e$),

$$\left.\frac{dE}{dt}\right|_{\text{e-ph}} = \frac{2\pi}{\hbar}\int_{BZ}\frac{\Omega d\mathbf{k}d\mathbf{k}'}{(2\pi)^6}\sum_{n'n\alpha}\delta(\varepsilon_{\mathbf{k}'n'}-\varepsilon_{\mathbf{k}n}-\hbar\omega_{\mathbf{k}'-\mathbf{k},\alpha}) \times \hbar\omega_{\mathbf{k}'-\mathbf{k},\alpha}\left|g^{\mathbf{k}'-\mathbf{k},\alpha}_{\mathbf{k}n,\mathbf{k}'n'}\right|^2 S(\varepsilon_{\mathbf{k}n},\varepsilon_{\mathbf{k}'n'},\omega_{\mathbf{k}'-\mathbf{k},\alpha}) \quad (1)$$

with

$$S(\varepsilon,\varepsilon',\omega) \equiv f(\varepsilon)n(\omega)(1-f(\varepsilon'))-(1-f(\varepsilon))(1+n(\omega))f(\varepsilon'). \quad (2)$$

Here $\Omega$ is the unit cell volume, $\varepsilon_{\mathbf{k}n}$ is the energy of electron with wave-vector $\mathbf{k}$ in band $n$, $\hbar\omega_{\mathbf{k}'-\mathbf{k},\alpha}$ is the energy of a phonon with wave-vector $\mathbf{q} = \mathbf{k}' - \mathbf{k}$ and polarization index $\alpha$, and $g^{\mathbf{k}'-\mathbf{k},\alpha}_{\mathbf{k}'n',\mathbf{k}n}$ is the *ab initio* electron-phonon matrix element coupling this phonon to electronic states indexed by $\mathbf{k}n$ and $\mathbf{k}'n'$. The band index explicitly includes spin as well in order to handle spinorial (relativistic) electronic states, and hence we do not include the conventional spin degeneracy factor present in non-relativistic expressions. (See Ref. 2 for more details.)

The above expressions involve double integrals over the Brillouin zone of *ab initio* electron-phonon matrix elements, and are expensive to evaluate even with the Wannier-function-based formulation that we use,[2] especially if we need to calculate it repeatedly (once per time step) for evaluating the collision integral in the Boltzmann equation. To arrive at a practical approximation which retains electronic structure details, we note that the phonon energy is negligible on the relevant electronic scale ($\hbar\omega \ll \varepsilon, \varepsilon'$). We can then Taylor expand the occupation factors in the energy-conserving cases of $S(\varepsilon, \varepsilon', \omega)$ (which are the only ones that contribute in (1) above) as

$$S(\varepsilon,\varepsilon+\hbar\omega,\omega) \approx -f(\varepsilon)(1-f(\varepsilon)) - \frac{\partial f}{\partial\varepsilon}\hbar\omega[1+n(\omega)-f(\varepsilon)] \quad (3)$$

Further, making the high-temperature phonon occupation factor approximation ($n(\omega) \approx k_BT_l/(\hbar\omega) \gg 1$)

shown to be highly accurate for calculating the total electron-phonon coupling strength in Ref. 3, we can simplify the above expression to

$$S(\varepsilon, \varepsilon + \hbar\omega, \omega) \approx -f(\varepsilon)(1 - f(\varepsilon)) - \frac{\partial f}{\partial \varepsilon} k_B T_l. \quad (4)$$

Now, we can substitute 4 and insert the identity $\int d\varepsilon \delta(\varepsilon - \varepsilon_{\mathbf{k}n})$ into (1), and rearrange it to collect contributions with same initial electron-energy

$$\left.\frac{dE}{dt}\right|_{\text{e-ph}} = -\int d\varepsilon H(\varepsilon) \left[ f(\varepsilon)(1 - f(\varepsilon)) + \frac{\partial f}{\partial \varepsilon} k_B T_l \right], \quad (5)$$

with the definition

$$H(\varepsilon) = \frac{2\pi}{\hbar} \int_{BZ} \frac{\Omega d\mathbf{k} d\mathbf{k}'}{(2\pi)^6} \sum_{n'n\alpha} \delta(\varepsilon - \varepsilon_{\mathbf{k}n}) \times \delta(\varepsilon_{\mathbf{k}'n'} - \varepsilon - \hbar\omega_{\mathbf{k}'-\mathbf{k},\alpha}) \hbar\omega_{\mathbf{k}'-\mathbf{k},\alpha} \left| g^{\mathbf{k}'-\mathbf{k},\alpha}_{\mathbf{k}n,\mathbf{k}'n'} \right|^2. \quad (6)$$

Finally, to calculate the electron-phonon contribution to the collision integral $\Gamma_{\text{e-ph}}[f(\varepsilon, t), T_l] = \left.\frac{df(\varepsilon)}{dt}\right|_{\text{e-ph}}$, we note that the contribution to $dE/dt$ from electrons with energy $\varepsilon$ corresponds to energy exchange between the lattice and electrons of energy $\varepsilon + \hbar\omega$, where $\hbar\omega$ is negligible on the energy scale of the electrons. Therefore we can equate the energy flow from the electrons to the lattice (the integrand in (5) above) to an energy flow from electrons with energy $\varepsilon$ to electrons with energy $\varepsilon + d\varepsilon$, resulting in the differential equation

$$-H(\varepsilon) \left[ f(\varepsilon)(1 - f(\varepsilon)) + \frac{\partial f}{\partial \varepsilon} k_B T_l \right] = \frac{\partial}{\partial \varepsilon} \left[ g(\varepsilon) \underbrace{\frac{df(\varepsilon)}{dt}}_{\Gamma_{\text{e-ph}}} \right], \quad (7)$$

where $g(\varepsilon)$ is the electronic density of states. Integrating by parts over $\varepsilon$ then yields the desired collision integral

$$\Gamma_{\text{e-ph}}[f(\varepsilon), T_l] = \frac{1}{g(\varepsilon)} \frac{\partial}{\partial \varepsilon} \left[ H(\varepsilon) \left( f(\varepsilon)(1 - f(\varepsilon)) + \frac{\partial f}{\partial \varepsilon} k_B T_l \right) \right], \quad (8)$$

which is the same as (4) in the main text.

In this approximate form, $H(\varepsilon)$ includes the detailed electronic structure, including energy dependence of the DFT-calculated density of states and electron-phonon matrix elements, but it only needs to be computed once for a material using the computationally-expensive (6). Subsequently, the collision integral given by (8) only involves a single integral over the electron energy which is computationally feasible for efficient solution of the Boltzmann equation. Appendix A presents a numerical tabulation of $H(\varepsilon)$ for the commonly used plasmonic metals, the noble metals and aluminum, which will be useful for implementing this efficient strategy in other analyses of pump probe spectroscopy of plasmonic metals.

Figure 1 plots $H(\varepsilon)$ for the noble metals and aluminum. Note that it varies by over two orders of magnitude with large increases below the Fermi level for noble metals due to $d$ bands, while aluminum exhibits only small variations. The shape of $H(\varepsilon)$ resembles the density of states $g(\varepsilon)$, but it is not strictly proportional to it because the involved electron-phonon matrix elements also vary with energy. We discuss this point at length in Ref. 1, where we plot the quantity $h(\varepsilon) \propto H(\varepsilon)/g(\varepsilon)$.

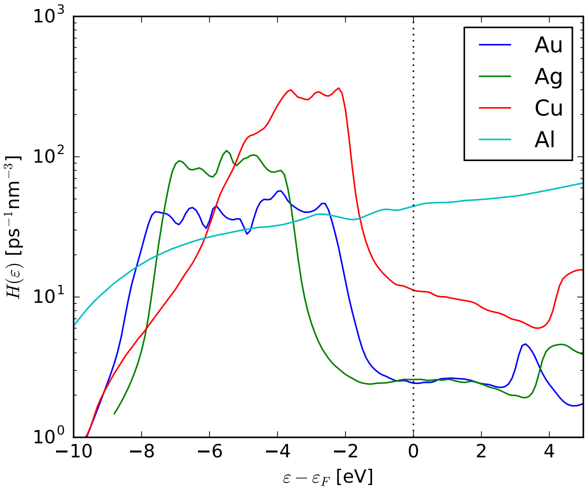


FIG. 1. *Ab initio* calculations of the energy-resolved electron-phonon coupling strength $H(\varepsilon)$ as a function of energy for the noble metals and aluminum, which allows retaining electronic-structure effects in the electron-phonon relaxation at low computational expense. See Appendix A for a numerical tabulation of these functions.


[1] A. M. Brown, R. Sundararaman, P. Narang, W. A. Goddard III, and H. A. Atwater, Phys. Rev. B **94**, 075120 (2016).

[2] A. Brown, R. Sundararaman, P. Narang, W. A. Goddard III, and H. A. Atwater, ACS Nano **10**, 957 (2016).

[3] Z. Lin and L. V. Zhigilei, Physical Review B , 075133 (2008).

## Appendix A: Numerical tabulation of $H(\varepsilon)$

| $\varepsilon - \varepsilon_F$ [eV] | $H(\varepsilon)$ [$ps^{-1}nm^{-3}$] Au | Ag | Cu | Al |
|---|---|---|---|---|
| -10.00 | 0.597480 | 0.000000 | 0.816735 | 6.198524 |
| -9.90 | 0.670881 | 0.000000 | 0.856266 | 6.689361 |
| -9.80 | 0.774425 | 0.000000 | 0.902880 | 7.187018 |
| -9.70 | 0.898215 | 0.000000 | 0.961690 | 7.703302 |
| -9.60 | 1.032793 | 0.000000 | 1.046594 | 8.235448 |
| -9.50 | 1.184179 | 0.000000 | 1.189638 | 8.765580 |
| -9.40 | 1.363770 | 0.000000 | 1.410654 | 9.294696 |
| -9.30 | 1.577994 | 0.000000 | 1.660172 | 9.808935 |
| -9.20 | 1.826637 | 0.000000 | 1.890825 | 10.321572 |
| -9.10 | 2.113965 | 0.000000 | 2.112152 | 10.842666 |
| -9.00 | 2.457445 | 0.000000 | 2.343315 | 11.405445 |
| -8.90 | 2.868770 | 0.000000 | 2.598360 | 12.008095 |
| -8.80 | 3.386541 | 1.475556 | 2.862264 | 12.595983 |
| -8.70 | 4.107117 | 1.618258 | 3.126024 | 13.145285 |
| -8.60 | 5.192705 | 1.786228 | 3.413060 | 13.684712 |
| -8.50 | 6.908772 | 1.986710 | 3.723084 | 14.266588 |
| -8.40 | 9.319275 | 2.230077 | 4.030691 | 14.860899 |
| -8.30 | 12.043378 | 2.531880 | 4.331233 | 15.458478 |
| -8.20 | 14.865087 | 2.916826 | 4.685048 | 16.055364 |
| -8.10 | 18.082123 | 3.427609 | 5.044037 | 16.612520 |
| -8.00 | 22.197636 | 4.148272 | 5.371962 | 17.192309 |
| -7.90 | 27.323185 | 5.268445 | 5.762644 | 17.790330 |
| -7.80 | 33.069582 | 7.184325 | 6.232967 | 18.385237 |
| -7.70 | 38.250519 | 10.484126 | 6.730229 | 18.943394 |
| -7.60 | 40.531103 | 15.844491 | 7.255323 | 19.462155 |
| -7.50 | 40.306331 | 23.601246 | 7.801365 | 19.988145 |
| -7.40 | 39.763118 | 33.675677 | 8.411933 | 20.522898 |
| -7.30 | 39.405506 | 46.299891 | 9.071933 | 21.033789 |
| -7.20 | 38.417504 | 61.757664 | 9.768299 | 21.546958 |
| -7.10 | 36.329505 | 77.907890 | 10.523777 | 22.063230 |
| -7.00 | 33.787195 | 88.939596 | 11.379665 | 22.524911 |
| -6.90 | 32.813062 | 93.446226 | 12.408457 | 22.967377 |
| -6.80 | 35.252292 | 92.037536 | 13.606140 | 23.426765 |
| -6.70 | 39.545822 | 86.882304 | 14.819928 | 23.907181 |
| -6.60 | 42.771785 | 81.543107 | 16.025767 | 24.383931 |
| -6.50 | 43.428595 | 80.743230 | 17.459897 | 24.839701 |
| -6.40 | 41.676827 | 81.827254 | 19.290432 | 25.273430 |
| -6.30 | 37.914873 | 83.165421 | 21.489945 | 25.677661 |
| -6.20 | 33.068636 | 80.826450 | 24.210219 | 26.062922 |
| -6.10 | 30.885413 | 76.448005 | 27.830557 | 26.463662 |
| -6.00 | 35.033425 | 72.838389 | 32.547644 | 26.861327 |
| -5.90 | 42.512403 | 71.883561 | 38.280315 | 27.198252 |
| -5.80 | 44.670602 | 76.628940 | 45.358527 | 27.488676 |
| -5.70 | 41.661348 | 90.777077 | 52.954444 | 27.797102 |
| -5.60 | 38.624055 | 103.900060 | 59.872873 | 28.141901 |
| -5.50 | 36.820101 | 110.604850 | 66.502617 | 28.477667 |
| -5.40 | 35.857701 | 105.218450 | 73.623761 | 28.807147 |
| -5.30 | 35.530336 | 90.396281 | 82.379442 | 29.146016 |
| -5.20 | 36.110198 | 86.604494 | 94.233431 | 29.483757 |
| -5.10 | 35.968756 | 91.477162 | 108.827669 | 29.828703 |
| -5.00 | 31.962004 | 96.512997 | 123.718213 | 30.138029 |
| -4.90 | 28.101706 | 98.116865 | 135.581203 | 30.396355 |
| -4.80 | 29.842037 | 101.840320 | 141.566473 | 30.646848 |
| -4.70 | 36.189737 | 103.235373 | 143.726323 | 30.976934 |
| -4.60 | 42.932975 | 101.059671 | 147.998533 | 31.302648 |
| -4.50 | 47.643976 | 93.836750 | 153.294295 | 31.499090 |
| -4.40 | 49.697666 | 86.398932 | 159.238665 | 31.547582 |
| -4.30 | 49.433814 | 81.130231 | 170.388386 | 31.643203 |
| -4.20 | 49.803150 | 78.124840 | 188.216701 | 31.864007 |
| -4.10 | 52.936707 | 77.546116 | 209.783632 | 32.114375 |

| $\varepsilon - \varepsilon_F$ [eV] | $H(\varepsilon)$ [$ps^{-1}nm^{-3}$] Au | Ag | Cu | Al |
|---|---|---|---|---|
| -4.00 | 56.637420 | 78.815377 | 231.675668 | 32.376151 |
| -3.90 | 57.186996 | 79.820041 | 253.170326 | 32.665279 |
| -3.80 | 53.446850 | 74.878951 | 274.375328 | 33.000097 |
| -3.70 | 48.705341 | 60.174976 | 292.369870 | 33.438294 |
| -3.60 | 45.743259 | 43.903692 | 299.672044 | 33.973505 |
| -3.50 | 43.877397 | 29.405280 | 281.384359 | 34.497851 |
| -3.40 | 42.289515 | 19.209973 | 265.960167 | 35.001015 |
| -3.30 | 40.984378 | 13.209101 | 262.028505 | 35.595797 |
| -3.20 | 40.247768 | 9.827595 | 256.885351 | 36.285612 |
| -3.10 | 40.237327 | 7.799188 | 254.971351 | 37.029560 |
| -3.00 | 40.701507 | 6.471954 | 266.348686 | 37.832214 |
| -2.90 | 41.660842 | 5.542253 | 283.624598 | 38.587687 |
| -2.80 | 43.653436 | 4.848347 | 290.475994 | 39.005172 |
| -2.70 | 46.340845 | 4.331875 | 283.355087 | 39.013894 |
| -2.60 | 46.431320 | 3.962417 | 273.305008 | 38.849016 |
| -2.50 | 41.809658 | 3.657115 | 270.749946 | 38.551685 |
| -2.40 | 34.813331 | 3.412770 | 279.261668 | 38.130836 |
| -2.30 | 28.241631 | 3.227020 | 296.272016 | 37.666112 |
| -2.20 | 22.429107 | 3.075512 | 308.724473 | 37.184839 |
| -2.10 | 17.106065 | 2.935300 | 283.311241 | 36.680719 |
| -2.00 | 12.882255 | 2.810574 | 216.920580 | 36.238897 |
| -1.90 | 9.923748 | 2.715421 | 139.326820 | 35.893158 |
| -1.80 | 7.845475 | 2.638158 | 83.873314 | 35.701858 |
| -1.70 | 6.309495 | 2.551878 | 54.253277 | 35.779615 |
| -1.60 | 5.119061 | 2.480718 | 39.054058 | 36.231247 |
| -1.50 | 4.263923 | 2.439441 | 30.371743 | 37.060418 |
| -1.40 | 3.717504 | 2.413600 | 24.933018 | 37.955130 |
| -1.30 | 3.380527 | 2.397134 | 21.328588 | 38.833731 |
| -1.20 | 3.151459 | 2.404588 | 18.811727 | 39.745956 |
| -1.10 | 2.989413 | 2.428734 | 17.076024 | 40.598065 |
| -1.00 | 2.863580 | 2.436585 | 15.837471 | 41.359983 |
| -0.90 | 2.778031 | 2.437883 | 14.817745 | 42.005387 |
| -0.80 | 2.720992 | 2.447703 | 14.017466 | 42.249750 |
| -0.70 | 2.648223 | 2.470743 | 13.302102 | 42.020193 |
| -0.60 | 2.574284 | 2.493939 | 12.686451 | 41.680184 |
| -0.50 | 2.525533 | 2.528236 | 12.257100 | 41.536025 |
| -0.40 | 2.523077 | 2.557014 | 12.105565 | 41.832011 |
| -0.30 | 2.542511 | 2.585195 | 12.021962 | 42.414980 |
| -0.20 | 2.522894 | 2.587301 | 11.740343 | 43.004344 |
| -0.10 | 2.470244 | 2.581560 | 11.451441 | 43.693398 |
| 0.00 | 2.435814 | 2.583180 | 11.200920 | 44.425385 |
| 0.10 | 2.426847 | 2.583427 | 11.034614 | 45.085237 |
| 0.20 | 2.436780 | 2.588506 | 10.984070 | 45.737887 |
| 0.30 | 2.464336 | 2.576051 | 10.923256 | 46.300993 |
| 0.40 | 2.463778 | 2.540278 | 10.881696 | 46.642588 |
| 0.50 | 2.464721 | 2.555209 | 10.751503 | 46.838757 |
| 0.60 | 2.495020 | 2.575880 | 10.415702 | 47.001483 |
| 0.70 | 2.559410 | 2.578451 | 10.146843 | 47.058244 |
| 0.80 | 2.614610 | 2.559763 | 10.053222 | 47.040557 |
| 0.90 | 2.623679 | 2.563904 | 10.052537 | 47.077239 |
| 1.00 | 2.630884 | 2.591037 | 9.973968 | 47.203988 |
| 1.10 | 2.642963 | 2.579932 | 9.841346 | 47.458961 |
| 1.20 | 2.634060 | 2.535060 | 9.741046 | 47.693959 |
| 1.30 | 2.620393 | 2.500295 | 9.654080 | 47.965374 |
| 1.40 | 2.620866 | 2.473010 | 9.540269 | 48.386402 |
| 1.50 | 2.604098 | 2.463454 | 9.465990 | 48.708489 |
| 1.60 | 2.577070 | 2.483351 | 9.371522 | 48.851114 |
| 1.70 | 2.543569 | 2.513114 | 9.260463 | 49.012515 |
| 1.80 | 2.496389 | 2.493051 | 9.079118 | 49.208001 |
| 1.90 | 2.450117 | 2.448111 | 8.805104 | 49.394081 |
| 2.00 | 2.416159 | 2.401856 | 8.480309 | 49.578514 |
| 2.10 | 2.396226 | 2.352809 | 8.237696 | 49.799448 |
| 2.20 | 2.383551 | 2.297894 | 8.031179 | 50.062242 |

| $\varepsilon - \varepsilon_F$ [eV] | $H(\varepsilon)$ [ps$^{-1}$nm$^{-3}$] | | | |
|---|---|---|---|---|
| | Au | Ag | Cu | Al |
| 2.30 | 2.348383 | 2.255700 | 7.898258 | 50.334948 |
| 2.40 | 2.304990 | 2.232271 | 7.810425 | 50.620405 |
| 2.50 | 2.276492 | 2.189032 | 7.704899 | 50.869306 |
| 2.60 | 2.271009 | 2.133390 | 7.566762 | 51.151426 |
| 2.70 | 2.303656 | 2.075882 | 7.378927 | 51.444578 |
| 2.80 | 2.403414 | 2.019139 | 7.153443 | 51.774267 |
| 2.90 | 2.631845 | 1.992539 | 6.967334 | 52.105309 |
| 3.00 | 3.095318 | 1.991042 | 6.871189 | 52.426393 |
| 3.10 | 3.862063 | 1.965651 | 6.784856 | 52.837046 |
| 3.20 | 4.511806 | 1.926301 | 6.650920 | 53.332478 |
| 3.30 | 4.628620 | 1.917617 | 6.459822 | 53.879606 |
| 3.40 | 4.404569 | 1.957138 | 6.255090 | 54.475118 |
| 3.50 | 4.069953 | 2.078739 | 6.106165 | 55.069544 |
| 3.60 | 3.649925 | 2.360859 | 6.008816 | 55.644777 |
| 3.70 | 3.212520 | 2.885108 | 6.009063 | 56.202618 |
| 3.80 | 2.850649 | 3.573692 | 6.112833 | 56.758981 |
| 3.90 | 2.583920 | 4.075775 | 6.350068 | 57.387389 |
| 4.00 | 2.385781 | 4.336034 | 6.838766 | 58.061439 |
| 4.10 | 2.220298 | 4.482171 | 7.942753 | 58.727943 |
| 4.20 | 2.064424 | 4.548858 | 9.876789 | 59.331686 |
| 4.30 | 1.927370 | 4.589624 | 12.049057 | 59.980713 |
| 4.40 | 1.815514 | 4.593069 | 13.493986 | 60.693005 |
| 4.50 | 1.737646 | 4.518367 | 14.244065 | 61.418616 |
| 4.60 | 1.694126 | 4.373779 | 14.762899 | 62.177836 |
| 4.70 | 1.676210 | 4.202975 | 15.175684 | 62.867071 |
| 4.80 | 1.681104 | 4.069866 | 15.490545 | 63.497082 |
| 4.90 | 1.703042 | 3.982175 | 15.635429 | 64.230583 |
| 5.00 | 1.745026 | 3.900388 | 15.587448 | 64.964196 |
